# Supplementary material for: SAGE-Nav: Leveraging LLM Planning and Alignment Fusion for Hierarchical Scene Graph-Guided Navigation
Source: arXiv:2606.25497 source file (2026-06-24)
Supplement: Supplementary file 1 [file 7_Appendix.tex]

\clearpage
\newpage

\makeatletter
\def\@captype{figure}
\makeatother

\setcounter{section}{0}
\setcounter{figure}{0}
\setcounter{table}{0}
\setcounter{equation}{0}

\section*{Appendix}
\addcontentsline{toc}{section}{Appendix}

\subsection{Scene Graph Construction}

To complement the brief description in the main manuscript, this section provides comprehensive details regarding the construction, hierarchical aggregation, and real-time maintenance of the Scene Graph used in SAGE-Nav.

\subsubsection{Incremental Node Instantiation and Update}
In contrast to the static pre-built graphs used during training, the deployment phase employs an incremental construction strategy. 
\begin{itemize}
    \item \textbf{Perception-to-Node Mapping:} At each time step $t$, the open-vocabulary detector extracts object instances from egocentric observations. Each detection is back-projected into the global 3D coordinate system using estimated depth and agent pose $p_t$.
    \item \textbf{Recursive Merging Mechanism:} To prevent node redundancy, a new detection $v_{new}$ is merged into an existing node $v_i$ if their Euclidean distance is within the threshold and they share the same semantic label. The node position $p_i$ is updated via a running average to mitigate localization jitter.
\end{itemize}

\subsubsection{Hierarchical Representation and Feature Encoding}
The SAGE-Nav framework organizes environmental knowledge into a multi-level Semantic Forest, enabling coarse-to-fine reasoning. As formalized in \textbf{Algorithm~\ref{alg:semantic_forest}}, this representation is constructed through a bottom-up abstraction process that transforms raw object instances into high-level area nodes.

\textbf{Multi-level Topological Structure.} Nodes $\mathcal{V}$ are categorized into three hierarchical levels: object, cluster, and area. Level $0$ contains atomic object instances $\mathcal{V}^0$ detected from observations. Higher levels ($\ell \ge 1$) are recursively generated using an agglomerative clustering mechanism based on spatial-semantic affinity. This structure ensures that the agent can maintain local geometric precision while performing long-horizon planning over topological regions.

\textbf{Unified Node Attributes.} To bridge perception and structure, each node $v_i$ is parameterized by a unified embedding $\mathbf{x}_i \in \mathbb{R}^{544}$, computed as:
\begin{equation}\mathbf{x}_i = [\mathbf{f}i ; \phi(\mathbf{q}i)],
\end{equation}
where $\mathbf{f}_i \in \mathbb{R}^{512}$ is the aggregated CLIP semantic feature and $\phi(\mathbf{q}_i) \in \mathbb{R}^{32}$ is the sinusoidal positional encoding of the 3D centroid $\mathbf{q}_i$. For parent nodes, $\mathbf{q}_{v_c}$ and $\mathbf{f}_{v_c}$ are derived via spatial and semantic mean-pooling of their constituent children nodes within cluster $C$, ensuring that higher-level abstractions remain representative of the underlying physical entities.

\textbf{Relational Connectivity.} Edges $\mathcal{E}$ define the information flow within the graph:
\begin{itemize}
\item \textbf{Hierarchical Edges} represent "part-of" containment relations, facilitating the distillation of global LLM plans into local waypoints.
\item \textbf{Intra-level Spatial Edges} are dynamically established between nodes at the same level if their Euclidean distance $\|\mathbf{q}_i - \mathbf{q}_j\|_2$ is below the threshold $\tau_s$. These edges provide the necessary context for the Relational Graph Convolutional Network (R-GCN) to capture local scene geometries and obstacle constraints.
\end{itemize}

\begin{algorithm}[t]
\caption{Hierarchical Scene Graph Generation (HSG)}
\label{alg:semantic_forest}
\small
\SetKwComment{Comment}{/* }{ */}
\KwIn{Initial object nodes $\mathcal{V}^0$ with spatial coordinates $\{\mathbf{q}_i\}$ and CLIP embeddings $\{\mathbf{f}_i\}$; max level $L$; clustering thresholds $\{\tau_\ell\}$; spatial threshold $\tau_s$}
\KwOut{Hierarchical scene graph $\mathcal{G}=(\mathcal{V},\mathcal{E})$}

Initialize $\mathcal{V}\leftarrow\mathcal{V}^0$, $\mathcal{E}\leftarrow\emptyset$, current level nodes $\mathcal{U}\leftarrow\mathcal{V}^0$\;

\For{$\ell=1$ \KwTo $L$}{
    \tcp{Hierarchical grouping via spatial-semantic clustering}
    $\mathcal{C}_\ell \leftarrow \text{AgglomerativeCluster}(\mathcal{U}, \tau_\ell)$\;
    $\mathcal{V}^\ell \leftarrow \emptyset$\;

    \ForEach{cluster $C \in \mathcal{C}_\ell$}{
        Create parent node $v_c$ (e.g., Area or Cluster node)\;
        \tcp{Feature Aggregation and Concatenation}
        $\mathbf{q}_{v_c} \leftarrow \text{Mean}(\{\mathbf{q}_i \mid v_i \in C\})$ \Comment*[r]{Spatial Centroid}
        $\mathbf{f}_{v_c} \leftarrow \text{Mean}(\{\mathbf{f}_i \mid v_i \in C\})$ \Comment*[r]{Semantic Mean}
        $\mathbf{x}_{v_c} \leftarrow [\mathbf{f}_{v_c} ; \phi(\mathbf{q}_{v_c})]$ \Comment*[r]{Unified Embedding}

        \tcp{LLM-based Knowledge Synthesis}
        $D(v_c) \leftarrow \text{LLMSummarize}(\{D(v_i) \mid v_i \in C\})$\;
        
        \tcp{Establish Hierarchical Containment Edges}
        \ForEach{$v_i \in C$}{
            $\mathcal{E} \leftarrow \mathcal{E} \cup \{(v_i, v_c, \text{is\_part\_of})\}$\;
        }
        $\mathcal{V}^\ell \leftarrow \mathcal{V}^\ell \cup \{v_c\}$; $\mathcal{V} \leftarrow \mathcal{V} \cup \{v_c\}$\;
    }

    \tcp{Establish Intra-level Spatial Relations}
    \ForEach{node pair $(v_i, v_j) \in \mathcal{V}^\ell$}{
        \If{$\|\mathbf{q}_i - \mathbf{q}_j\|_2 \le \tau_s$}{
            $r_{ij} \leftarrow \text{SpatialRelation}(\mathbf{q}_i, \mathbf{q}_j)$\;
            $\mathcal{E} \leftarrow \mathcal{E} \cup \{(v_i, v_j, r_{ij})\}$\;
        }
    }
    $\mathcal{U} \leftarrow \mathcal{V}^\ell$ \Comment*[r]{Iterate to next abstraction level}
}
\Return{$\mathcal{G}$}
\end{algorithm}

\subsubsection{Task-relevant Subgraph Extraction}
To facilitate efficient LLM reasoning, we implement a multi-stage retrieval cascade to extract a compact subgraph $\mathcal{G}_Q$:
\begin{enumerate}
    \item \textbf{Semantic Pre-filtering:} Nodes are ranked by cosine similarity between their CLIP embeddings and the target query $q$.
    \item \textbf{Contextual Augmentation:} The score of each node is weighted by the relevance of its ancestral chain (Area and Cluster levels) using a hierarchical gain factor $\beta_h$.
    \item \textbf{Spatial Boosting:} Top-ranked nodes are further refined by the scores of their spatial neighbors to prioritize topologically significant waypoints.
\end{enumerate}
\begin{figure}[H]
    \centering
    \includegraphics[width=1.0\columnwidth]{figures/subgraph_extraction.png}
    \caption{
        System prompt for hierarchical path generation.
}
    \label{fig:hsge}
    \vspace{-0.8em}
\end{figure}

\subsection{LLM Global Planner}

\subsection{Training Implementation Details}
This section expands upon the training protocols, optimization objectives, and simulation configurations to ensure the reproducibility of SAGE-Nav.

\subsubsection{Loss Function Decomposition}
SAGE-Nav is optimized using the Asynchronous Advantage Actor-Critic (A3C) framework. The total loss $\mathcal{L}_{total}$ is decomposed into three synergistic components:
\begin{equation}
    \mathcal{L}_{total} = \mathcal{L}_{policy} + \lambda_{v}\mathcal{L}_{value} + \lambda_{e}\mathcal{L}_{entropy}
\end{equation}
where:
\begin{itemize}
    \item \textbf{Policy Loss ($\mathcal{L}_{policy}$):} To minimize variance during gradient estimation, we utilize the advantage function $A_t = R_t - V(s_t)$, formulated as:
    \begin{equation}
        \mathcal{L}_{policy} = -\mathbb{E}_t[\log \pi(a_t|s_t) \cdot A_t]
    \end{equation}
    where $R_t$ represents the $n$-step discounted return.
    \item \textbf{Value Loss ($\mathcal{L}_{value}$):} We employ the Mean Squared Error (MSE) to align the critic's estimation $V(s_t)$ with the empirical return $R_t$:
    \begin{equation}
        \mathcal{L}_{value} = \mathbb{E}_t[(R_t - V(s_t))^2]
    \end{equation}
    \item \textbf{Entropy Regularization ($\mathcal{L}_{entropy}$):} To prevent premature convergence to suboptimal deterministic policies, an entropy term $H(\pi)$ is added:
    \begin{equation}
        \mathcal{L}_{entropy} = \mathbb{E}_t[H(\pi(\cdot|s_t))]
    \end{equation}
    The coefficient $\lambda_e$ is set to $1 \times 10^{-2}$  to maintain sufficient environmental exploration.
\end{itemize}

\subsubsection{Curriculum Design and Scheduling}
The training process follows a structured curriculum to stabilize the high-dimensional alignment in GAFN:
\begin{enumerate}
    \item \textbf{Feature Initialization:} The visual backbone (ResNet-18) and Language Encoder (CLIP) are frozen to provide stable semantic anchors.
    \item \textbf{Warm-up Phase:} During the initial $1 \times 10^6$ episodes, the agent focuses on local obstacle avoidance and basic scene graph navigation.
    \item \textbf{Learning Rate Decay:} We utilize the Adam optimizer with an initial learning rate $\eta = 1 \times 10^{-4}$. Upon reaching $3 \times 10^6$ episodes, $\eta$ is decayed to $1 \times 10^{-5}$ to facilitate fine-grained policy refinement.
\end{enumerate}

\subsubsection{Simulator Configuration (AI2-THOR)}
For consistent evaluation across i-THOR and RoboTHOR, we enforce the following constraints:
\begin{itemize}
    \item \textbf{Success Criteria:} An episode is terminated as \texttt{Success} only if the target is within the agent's field of view and the Euclidean distance $d \le 1.5$m.
    \item \textbf{Environmental Randomization:} To enhance generalization, the agent's starting pose $(x, y, \theta_{yaw})$ and target object instances are randomized at the start of each episode.
    \item \textbf{Hardware Scalability:} Training is executed across 4 NVIDIA RTX 3090 GPUs, utilizing 16 asynchronous workers to maximize throughput while maintaining gradient consistency.
\end{itemize}

\subsection{Detailed Hyperparameter Table}
\begin{table*}[t]
\centering
\caption{Nomenclature and Parameter Definitions for SAGE-Nav}
\label{tab:supp_params}
\small

\begin{tabular}{lp{3cm}p{7.5cm}l}
\hline
\textbf{Notation} & \textbf{Type / Unit} & \textbf{Description} & \textbf{Value} \\
\hline
$t$ & Number & Discrete time step in navigation episode & - \\
$c$ & String & Category of the target object query & - \\
$\mathcal{I}_t^{rgb}$ & Matrix ($640 \times 480 \times 3$) & RGB image observed by the agent at time $t$  & - \\
$p_t$ & $\langle x, z, \theta_{yaw}, \theta_{pitch} \rangle$ & Current pose of agent (AI2-THOR planar coordinates and orientation)  & - \\
$v_i$ & Node & An entity node in $\mathcal{G}$, representing an object, cluster, or area  & - \\
$\mathcal{G}$ & $\langle \mathcal{V}, \mathcal{E} \rangle$ & Hierarchical scene graph composed of nodes and edges  & - \\
\hline
$R_{success}$ & Number & Sparse reward for successful goal reaching ($D_{agent, target} \le d_s$) & 5.0 \\
\hline
$D_{cluster}$ & Meter (m) & Spatial threshold ($\tau_\ell, \tau_s$) for recursive node merging and adjacency & 2.0 \\
$S_{merge}$ & Scalar $\in [0,1]$ & Semantic similarity threshold ($\alpha$) for node aggregation & 0.6 \\
$\delta$ & Scalar $\in [0,1]$ & Cosine similarity threshold for waypoint completion & 0.7 \\
$d_s$ & Meter (m) & Euclidean distance threshold for success termination & 1.5 \\
\hline
$\kappa$ & Scalar & GAFN gate sensitivity scaling factor in $\lambda$ formulation & 2.0 \\
$\tau$ & Scalar & GAFN visual preservation coefficient for feature weighting & 0.5 \\
$g$ & Scalar & Predicted gating scale via MLP in GAFN & - \\
$\mathbf{f}_{CLIP}$ & Vector ($\mathbb{R}^{512}$) & Frozen CLIP-ViT-B/32 semantic embedding for visual features & 512-dim \\
$\mathbf{q}_i$ & Vector ($\mathbb{R}^{3}$) & Global 3D coordinates of node $v_i$ & - \\
$\phi(\mathbf{q})$ & Vector ($\mathbb{R}^{32}$) & Sinusoidal positional encoding of node coordinates & 32-dim \\
$d_{in}$ & Number & Input dimension of HSGE (Concatenation of $[\mathbf{f}; \phi(\mathbf{q})]$) & 544 \\
$d_{hid}$ & Number & Hidden dimension of the 3-layer R-GCN and GAFN & 128 \\
$d_{out}$ & Number & Final dimension of fused feature $\mathbf{F}_f$ & 64 \\
$h_t$ & Vector ($\mathbb{R}^{512}$) & Hidden state of the navigation policy LSTM & 512-dim \\
\hline 
\end{tabular}
\end{table*}

The detailed hyperparameter configuration is summarized in Table \ref{tab:supp_params}. In our reinforcement learning setup, $R_t, R_p, R_a,$ and $\lambda$ denote the success reward, step penalty, exploration reward, and distance scaling factor, respectively. For network architecture, $d_{hid}$ and $d_{out}$ represent the hidden and output dimensions of the R-GCN layers within the HSGE. Regarding scene graph construction, $D_{cluster}$ defines the spatial merging radius, $S_{merge}$ is the semantic similarity threshold, and $E_{dist}$ specifies the maximum distance for edge connectivity. In the execution phase, the waypoint transition is governed by the similarity gate $\delta$ and the success threshold $d_s$

\subsection{Ablation Studies}
\begin{table}[H]
\centering
\caption{ABLATION STUDY AND PARAMETER SENSITIVITY ANALYSIS}
\label{table:ablation_analysis}
\resizebox{\columnwidth}{!}{
\begin{tabular}{l|l|ccc} 
\toprule
\textbf{Group} & \textbf{Variant Configuration} & \textbf{SR$\uparrow$(\%)} & \textbf{SPL$\uparrow$(\%)} & \textbf{DTS$\downarrow$(m)} \\ \midrule
\multicolumn{2}{l|}{\textbf{SAGE-Nav (Default Setting)$^{\ast}$}} & \textbf{82.47} & \textbf{42.34} & \textbf{0.32} \\ \midrule
\multirow{3}{*}{$\lambda_{align}$} & $\lambda = 0.1$ & 81.95 & 41.80 & 0.35 \\
 & $\lambda = 0.5$ & 82.10 & 42.05 & 0.34 \\
 & $\lambda = 0.7$ & 80.85 & 40.92 & 0.37 \\ \midrule
Strategy & Frozen HSGE  & 81.25 & 40.98 & 0.38 \\ \midrule
Hierarchy & Flat SG & 80.50 & 39.76 & 0.38 \\ \midrule
% \multicolumn{5}{l}{\textit{5) Generalization (Default: In-domain)}} \\ \midrule
General. & Zero-shot (RoboTHOR) &  &  &  \\ \bottomrule
\end{tabular}
}
\vspace{-1.0em}
\scriptsize{\raggedright $^{\ast}$Default Setting: $\lambda=0.3$, End-to-End Training, Hierarchical SG. \par}
\end{table}
Beyond the primary module ablations, we executed extended experiments to validate the robustness of our framework across varying parametric and structural conditions. These evaluations focus on the system's sensitivity to alignment-guided feedback and its cross-simulator generalization capabilities, providing a comprehensive assessment of the model's reliability in complex embodied environments.Table \ref{table:ablation_analysis} demonstrates that our method is insensitive to variations in $\lambda_{align}$, maintaining consistent performance across $\lambda \in [0.1, 0.5]$. This stability indicates that the policy benefits from the intrinsic structural guidance without requiring precise hyperparameter calibration.

\subsection{Extended Visualizations}
\subsection{Pseudocode}
\begin{algorithm}[t]
\caption{Overall Pipeline of SAGE-Nav}
\label{alg:sage_nav}
\small

\KwIn{Target category $g$, RGB-D observation $\mathcal{I}_t$, initial graph $\mathcal{G}$}
\KwOut{Action $a_t$, Task completion status}

\tcp{Stage 1: Offline/Online Global Prior Construction}
\If{Mode = Offline}{
    \tcp{Build full graph once}
    $\mathcal{M}_t \leftarrow \bluekw{OpenSeeD}(\mathcal{I}_t)$; \hfill $\triangleright$ Instance Segmentation \\
    $f_i \leftarrow \bluekw{CLIP}(\text{crops})$; \hfill $\triangleright$ Node Embedding \\
    $\mathcal{G} \leftarrow \bluekw{ProjectTo3D}(\mathcal{M}_t, d_t, p_t)$; \hfill $\triangleright$ Spatial Mapping \\
}
\Else{
    \tcp{Online warm-up for initial graph}
    \For{$t=1$ \KwTo $T_{\text{init}}$}{
        $\mathcal{M}_t \leftarrow \bluekw{OpenSeeD}(\mathcal{I}_t)$; \\
        $\mathcal{C}_t \leftarrow \bluekw{ProjectTo3D}(\mathcal{M}_t, d_t, p_t)$; \\
        $\mathcal{G} \leftarrow \bluekw{UpdateGraph}(\mathcal{G}, \mathcal{C}_t)$; \\
    }
}

\tcp{Stage 2: LLM-Guided Global Planning (H-GP)}
$\mathcal{P}^* \leftarrow \bluekw{LLMGlobalPlanner}(\mathcal{G}, g)$; \hfill $\triangleright$ Sec. IV-B \\
Initialize waypoint queue $\mathcal{Q} \leftarrow \{w_1, \dots, w_T\}$;

\tcp{Stage 3: Online Execution with Incremental Mapping}
\Repeat{$a_t$ is \texttt{Done}}{
    \tcp{Online Graph Update (Incremental Mapping)}
    $\mathcal{M}_t^{new} \leftarrow \bluekw{OpenSeeD}(\mathcal{I}_t)$; \\
    $\mathcal{C}_t \leftarrow \bluekw{ProjectTo3D}(\mathcal{M}_t^{new}, d_t, p_t)$; \hfill $\triangleright$ 3D Candidates \\
    $\mathcal{A}_t \leftarrow \bluekw{Associate}(\mathcal{C}_t, \mathcal{G})$; \hfill $\triangleright$ Data Association \\
    \ForEach{$c_i \in \mathcal{C}_t$}{
        \lIf{$c_i \in \mathcal{A}_t$}{\bluekw{UpdateNode}($v, c_i$)} \tcp*[f]{EMA fusion}
        \lElse{$\mathcal{G} \leftarrow \mathcal{G} \cup \{v_{new}\}$} \tcp*[f]{Create new node}
    }
    $\mathcal{G} \leftarrow \bluekw{PruneMerge}(\mathcal{G})$; \hfill $\triangleright$ Maintenance \\

    \tcp{Optional Re-planning}
    \If{\texttt{GraphUpdated} \textbf{or} \texttt{WaypointFailed}}{
        $\mathcal{P}^* \leftarrow \bluekw{LLMGlobalPlanner}(\mathcal{G}, g)$; \\
        Update $\mathcal{Q}$;
    }

    \tcp{Hierarchical Feature Fusion}
    $F_{img} \leftarrow \bluekw{ResNet18}(\mathcal{I}_t)$; \hfill $\triangleright$ Visual perception \\
    $h_{global} \leftarrow \bluekw{HSGE}(\mathcal{G}_{sub}, w_i)$; \hfill $\triangleright$ Sec. IV-C \\

    \tcp{Alignment and Waypoint Switching}
    $\alpha_t \leftarrow \bluekw{ComputeAlignment}(F_{img}, w_i)$; \hfill $\triangleright$ Eq. (9) \\
    \If{$\alpha_t \ge \delta$ \textbf{and} $\text{dist} \le d_s$}{
        $w_i \leftarrow \bluekw{Pop}(\mathcal{Q})$; \hfill $\triangleright$ Progress waypoint \\
    }

    \tcp{Decision Making via GAFN}
    $F_f \leftarrow \bluekw{GAFN}(F_{img}, h_{global}, w_i, \alpha_t)$; \hfill $\triangleright$ Sec. IV-D \\
    $a_t, h_{t+1} \leftarrow \bluekw{ActorCritic}(F_f, h_t)$; \hfill $\triangleright$ A3C Policy \\
    Execute $a_t$ in environment;
}
\end{algorithm}

\subsection{Real-world Setup}
\subsection{RGCN Encoder}

\begin{figure}[t]
  \centering
  
  \includegraphics[width=1.0\linewidth]{figures/heatmap.png} 
  \vspace{-2mm} 
  \caption{
  \textbf{Robustness Analysis under Varying Occlusion Rates.} 
  The top histogram illustrates the difficulty distribution of the test set, showing a long-tail distribution with high-occlusion scenarios. 
  The bottom heatmap compares the Success Rate (SR) of \textbf{SAGE-Nav (Ours)} against baselines across these intervals. 
  Our method demonstrates superior robustness, particularly in the challenging \textbf{80\%--95\%} occlusion range (where the majority of hard cases reside), maintaining a high SR while baselines degrade significantly.
  $^*$Note: The sample count in the 95--100\% bin is extremely low ($N<10$), resulting in high statistical variance.
  }
  \label{fig:occlusion_heatmap}
  \vspace{-4mm} 
\end{figure}

\begin{figure}[t]
    \centering
    \includegraphics[width=1.0\columnwidth]{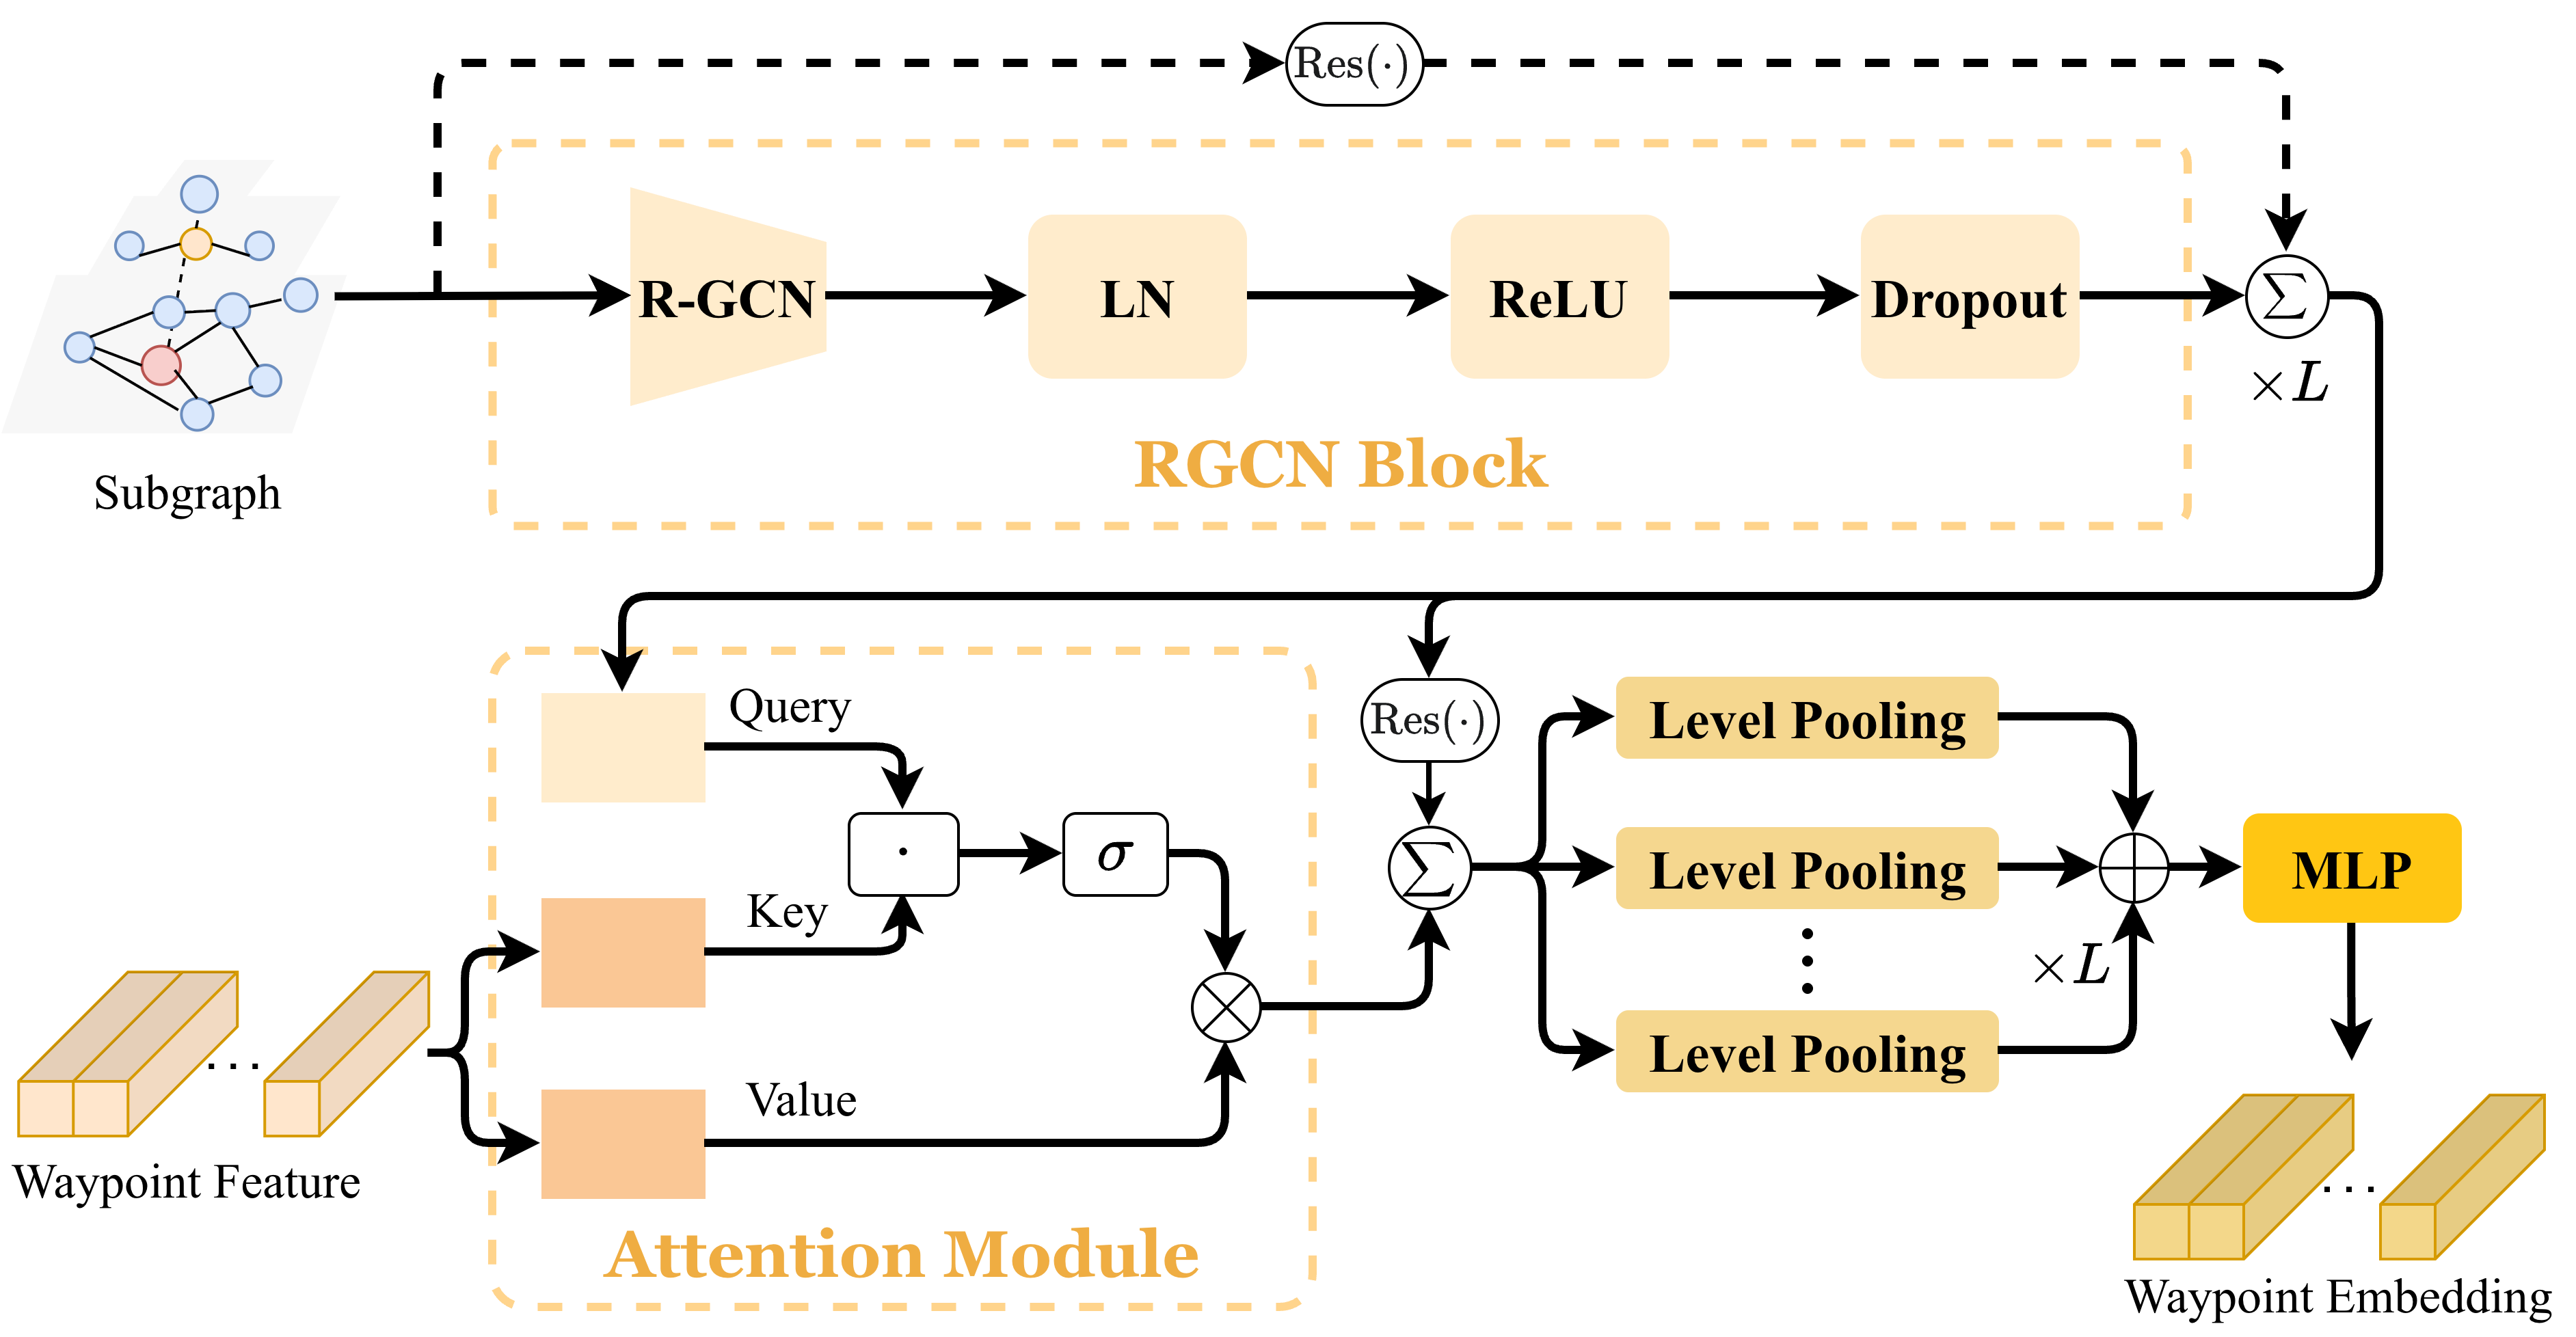}
    \caption{
        The HSGE processes Subgraph structure, Node Features, and a Goal Feature to generate a robust Waypoint Feature. The architecture consists of three main stages: 
        (1) RGCN Encoder with global $\text{Res}(\cdot)$, (2) Attention Module for goal infusion, and (3) Level Pooling followed by hierarchical fusion and dynamic selection ($\text{WP Selector}$).
}
    \label{fig:hsge}
    \vspace{-0.8em}
\end{figure}
